# Supplementary material for: Adapting Rapid Motor Adaptation for Bipedal Robots
Source: arXiv:2205.15299 source file (2022-09-06)
Supplement: Supplementary file 1 [file supplementary.tex]

\begin{figure*}
\begin{subfigure}{.24\linewidth}
  \centering
  \includegraphics[width=\linewidth]{figures/flat_ground.pdf}
  \caption{flat}
  \label{fig:flat-ground-comp}
\end{subfigure}
\begin{subfigure}{.24\linewidth}
  \centering
  \includegraphics[width=\linewidth]{figures/slippery_ground.pdf}
  \caption{slippery}
  \label{fig:slippery-ground-comp}
\end{subfigure}
\begin{subfigure}{.24\linewidth}
  \centering
  \includegraphics[width=\linewidth]{figures/foam_ground.pdf}
  \caption{foam}
  \label{fig:foam-ground-comp}
\end{subfigure}
\begin{subfigure}{.24\linewidth}
  \centering
  \includegraphics[width=\linewidth]{figures/load_lifting.pdf}
  \caption{load}
  \label{fig:load-lifting-comp}
\end{subfigure}
\caption{\zli{Not sure we should demonstrate this}}
\end{figure*}

\begin{figure*}
\begin{subfigure}{.24\linewidth}
  \centering
  \includegraphics[width=\linewidth]{figures/flat_ground_pp.pdf}
  \caption{flat}
  \label{fig:flat-ground-pp}
\end{subfigure}
\begin{subfigure}{.24\linewidth}
  \centering
  \includegraphics[width=\linewidth]{figures/slippery_ground_pp.pdf}
  \caption{slippery}
  \label{fig:slippery-ground-pp}
\end{subfigure}
\begin{subfigure}{.24\linewidth}
  \centering
  \includegraphics[width=\linewidth]{figures/foam_ground_pp.pdf}
  \caption{foam}
  \label{fig:foam-ground-pp}
\end{subfigure}
\begin{subfigure}{.24\linewidth}
  \centering
  \includegraphics[width=\linewidth]{figures/load_lifting_pp.pdf}
  \caption{load}
  \label{fig:load-lifting-pp}
\end{subfigure}
\caption{Phase portrait, \zli{Not sure we should demonstrate this}}
 \end{figure*}
